# Supplementary material for: Edge Impulse: An MLOps Platform for Tiny Machine Learning
Source: arXiv:2212.03332 source file (2023-04-28)
Supplement: Supplementary file 1 [file appendix.tex]

\appendix

\section{Appendix}
